# Supplementary material for: Electromagnetic helicity in complex media
Source: arXiv:1802.09392 ancillary file (2018-05-07)
Supplement: Supplementary file 1 [file Helicity_Supplemental_Material.pdf]

# Supplemental Material: Electromagnetic Helicity in Complex Media

F. Alpegiani,<sup>1</sup> K. Y. Bliokh,<sup>2,3</sup> F. Nori,<sup>2,4</sup> and L. Kuipers<sup>1</sup>

<sup>1</sup>*Department of Quantum Nanoscience, Kavli Institute of Nanoscience Delft,  
Delft University of Technology, Lorentzweg 1, 2628 CJ Delft, The Netherlands*

<sup>2</sup>*Theoretical Quantum Physics Laboratory, RIKEN Cluster for Pioneering Research, Wako-shi, Saitama 351-0198, Japan*

<sup>3</sup>*Nonlinear Physics Centre, RSPE, The Australian National University, Canberra, Australia*

<sup>4</sup>*Physics Department, University of Michigan, Ann Arbor, Michigan 48109-1040, USA*

## BI-ORTHOGONAL ELECTROMAGNETISM

Here we derive the bi-orthogonal (non-Hermitian) Hamiltonian formalism for Maxwell equations, Eqs. (1)–(3) of the main text. We use an approach similar to Refs. [1–4].

The starting point is to express the frequency-dependent permittivity matrix [Eq. (2) in the main text] in the following expansion form [2]:

$$M(\omega) = M_\infty + \sum_\alpha \frac{M_\alpha}{\omega - \omega_\alpha}, \quad (1)$$

where  $M_\alpha$  is the matrix residual at the pole  $\omega = \omega_\alpha$ , and here we omit the hats over the matrices. Since we are considering lossless media, the operator  $M(\omega)$  is Hermitian and all the pole frequencies  $\omega_\alpha$  are real [2]. The basic idea is to reduce Maxwell equations [Eq. (1) in the main text] into a Schrödinger-like form by defining the set of six-component supplemental fields:

$$\mathbf{q}_\alpha = \frac{\omega_\alpha}{\omega - \omega_\alpha} \begin{pmatrix} \mathbf{E} \\ \mathbf{H} \end{pmatrix} \equiv \frac{\omega_\alpha}{\omega - \omega_\alpha} \mathbf{f}. \quad (2)$$

Temporarily diverging from the notation used in the main text, we denote the electromagnetic bispinor  $(\mathbf{E}, \mathbf{H})^T$  by the symbol  $\mathbf{f}$ . Note that our definition of the supplemental fields is different from Ref. [2].

With the introduction of the supplemental fields, Eq. (1) in the main text becomes:

$$\begin{pmatrix} \mathcal{H}_0 & -M_\infty^{-1}M_1 & -M_\infty^{-1}M_2 & \dots \\ \omega_1 & \omega_1 & 0 & \dots \\ \omega_2 & 0 & \omega_2 & \dots \\ \vdots & \vdots & \vdots & \ddots \end{pmatrix} \begin{pmatrix} \mathbf{f} \\ \mathbf{q}_1 \\ \mathbf{q}_2 \\ \vdots \end{pmatrix} = \omega \begin{pmatrix} \mathbf{f} \\ \mathbf{q}_1 \\ \mathbf{q}_2 \\ \vdots \end{pmatrix}, \quad (3)$$

where

$$\mathcal{H}_0 = M_\infty^{-1} \begin{pmatrix} 0 & i\nabla \times \\ -i\nabla \times & 0 \end{pmatrix} - \sum_\alpha M_\infty^{-1}M_\alpha. \quad (4)$$

Equation (3) represents a linear eigenvalue problem, with the frequency eigenvalue  $\omega$  in the right-hand side.

The Hamiltonian in Eq. (3) is not Hermitian with respect to the standard inner product. According to the prescriptions of biorthogonal quantum mechanics [5], each right eigenvector  $\mathbf{W} = (\mathbf{f}, \mathbf{q}_1, \mathbf{q}_2, \dots)^T$  has the left eigenvector partner  $\tilde{\mathbf{W}} = (\tilde{\mathbf{f}}, \tilde{\mathbf{q}}_1, \tilde{\mathbf{q}}_2, \dots)^T$ , which is the solution of the eigenvalue problem for the Hermitian-conjugate Hamiltonian:

$$\begin{pmatrix} \mathcal{H}_0^\dagger & \omega_1 & \omega_2 & \dots \\ -M_1M_\infty^{-1} & \omega_1 & 0 & \dots \\ -M_2M_\infty^{-1} & 0 & \omega_2 & \dots \\ \vdots & \vdots & \vdots & \ddots \end{pmatrix} \begin{pmatrix} \tilde{\mathbf{f}} \\ \tilde{\mathbf{q}}_1 \\ \tilde{\mathbf{q}}_2 \\ \vdots \end{pmatrix} = \omega \begin{pmatrix} \tilde{\mathbf{f}} \\ \tilde{\mathbf{q}}_1 \\ \tilde{\mathbf{q}}_2 \\ \vdots \end{pmatrix}. \quad (5)$$

Here, we have used the assumption that  $M_\infty$  and  $M_\alpha$  are Hermitian matrices. This fact stems directly from the restriction to lossless media and the corresponding conditions on the permittivity matrix  $M(\omega)$ .

Expressing  $\tilde{\mathbf{q}}_\alpha$  from the lower equations of the set (5),  $\tilde{\mathbf{q}}_\alpha = -M_\alpha M_\infty^{-1} \tilde{\mathbf{f}} / (\omega - \omega_\alpha)$ , and substituting it into the first Eq. (5), we obtain:

$$\begin{pmatrix} 0 & i\nabla \times \\ -i\nabla \times & 0 \end{pmatrix} M_\infty^{-1} \tilde{\mathbf{f}} = \omega \left[ M_\infty + \sum_\alpha \frac{M_\alpha}{\omega - \omega_\alpha} \right] M_\infty^{-1} \tilde{\mathbf{f}}. \quad (6)$$

Comparing this equation with the original Maxwell's equations, we immediately find:

$$\tilde{\mathbf{f}} = M_\infty \mathbf{f}, \quad \tilde{\mathbf{q}}_\alpha = -\frac{M_\alpha}{\omega - \omega_\alpha} \mathbf{f}. \quad (7)$$

Next, for an operator  $\hat{O}$ , it is natural to define the local expectation value using the biorthogonal pair of the “extended” eigenvectors  $\mathbf{W} = (\mathbf{f}, \mathbf{q}_1, \mathbf{q}_2, \dots)^T$  and  $\tilde{\mathbf{W}} = (\tilde{\mathbf{f}}, \tilde{\mathbf{q}}_1, \tilde{\mathbf{q}}_2, \dots)^T$ :

$$O = g \operatorname{Re} \left( \tilde{\mathbf{W}}^\dagger \hat{O} \mathbf{W} \right) = g \operatorname{Re} \left( \tilde{\mathbf{f}}^\dagger \hat{O} \mathbf{f} + \sum_\alpha \tilde{\mathbf{q}}_\alpha^\dagger \hat{O} \mathbf{q}_\alpha \right). \quad (8)$$

Substituting here Eqs. (2) and (7), we derive Eq. (4) of the main text:

$$O = g \operatorname{Re} \left[ (M_\infty \mathbf{f})^\dagger \hat{O} \mathbf{f} - \sum_\alpha \frac{\omega_\alpha}{(\omega - \omega_\alpha)^2} (M_\alpha \mathbf{f})^\dagger \hat{O} \mathbf{f} \right] = g \operatorname{Re} \left( \tilde{\psi}^\dagger \hat{O} \psi \right), \quad (9)$$

where the bispinor  $\psi = \mathbf{f} = (\mathbf{E}, \mathbf{H})^T$  (recovering the notation of the main text), and the adjoint bispinor reads:

$$\tilde{\psi} = \left( M_\infty - \sum_\alpha \frac{\omega_\alpha}{(\omega - \omega_\alpha)^2} M_\alpha \right) \mathbf{f} = \frac{\partial [\omega M(\omega)]}{\partial \omega} \begin{pmatrix} \mathbf{E} \\ \mathbf{H} \end{pmatrix}. \quad (10)$$

This result is exactly equivalent to Eq. (3) in the main text. Note that, in order to derive Eq. (9), it is essential to use a biorthogonal basis where the medium parameters appear explicitly only in the adjoint eigenvector  $\tilde{\psi}$ , as opposed, for instance, to a different choice of the basis where the medium parameters are symmetrized between  $\psi$  and  $\tilde{\psi}$ . This condition ensures that the medium parameters are not subject to the action of the operator  $\hat{O}$ .

## HELICITY DENSITY AND CONSERVATION IN THE TIME DOMAIN

The Hamiltonian formulation of electromagnetism that we have described in the previous section and extensively used in the main text is naturally formulated in the frequency domain, as it is based on describing the fields as frequency eigenmodes of an effective Hamiltonian. Here we introduce a time-domain expression for the helicity density and its conservation law (continuity equation), which reduces to the frequency-domain helicity density presented in the main text in the case of monochromatic fields. In this section, we mostly use the approach suggested by Philbin [6].

Following Ref. [6], we write the permittivity and the permeability as series expansions in the frequency variable, and we convert them to time-dependent differential operators using the  $\omega \rightarrow i\partial_t$  replacement:

$$\begin{aligned} \varepsilon(\mathbf{r}, \omega) &= \sum_n \varepsilon_{2n}(\mathbf{r}) \omega^{2n} \longrightarrow \varepsilon(\mathbf{r}, i\partial_t) = \sum_n \varepsilon_{2n}(\mathbf{r}) i^{2n} \frac{\partial^{2n}}{\partial t^{2n}}, \\ \mu(\mathbf{r}, \omega) &= \sum_n \mu_{2n}(\mathbf{r}) \omega^{2n} \longrightarrow \mu(\mathbf{r}, i\partial_t) = \sum_n \mu_{2n}(\mathbf{r}) i^{2n} \frac{\partial^{2n}}{\partial t^{2n}}. \end{aligned} \quad (11)$$

We consider the time-dependent electric and magnetic fields and displacements,  $\mathcal{E}(\mathbf{r}, t)$ ,  $\mathcal{H}(\mathbf{r}, t)$ ,  $\mathcal{D}(\mathbf{r}, t)$ , and  $\mathcal{B}(\mathbf{r}, t)$ , satisfying Maxwell's equations in the time domain, as well as the vector-potentials  $\mathcal{A}(\mathbf{r}, t)$  and  $\mathcal{C}(\mathbf{r}, t)$ , which are related to the fields as:

$$\mathcal{B} = \nabla \times \mathcal{A}, \quad \mathcal{D} = -\nabla \times \mathcal{C}, \quad \mathcal{E} = -\partial_t \mathcal{A}, \quad \mathcal{H} = -\partial_t \mathcal{C}. \quad (12)$$

It is always possible to define the potentials in this way in the absence of free charges because  $\mathcal{D}$  and  $\mathcal{B}$  are solenoidal fields.

We also introduce the modified potentials

$$\mathcal{A}'(\mathbf{r}, t) = \nu(\mathbf{r}, i\partial_t) Z^{-1}(\mathbf{r}, i\partial_t) \mathcal{A}(\mathbf{r}, t), \quad \mathcal{C}'(\mathbf{r}, t) = \nu(\mathbf{r}, i\partial_t) Z(\mathbf{r}, i\partial_t) \mathcal{C}(\mathbf{r}, t), \quad (13)$$

where  $Z(\mathbf{r}, i\partial_t)$  and  $\nu(\mathbf{r}, i\partial_t)$  correspond to the optical impedance  $Z(\mathbf{r}, \omega)$  and the phase factor  $\nu(\mathbf{r}, \omega)$  defined in the main text. Note that the products  $\nu(\omega)Z(\omega)$  and  $\nu(\omega)Z^{-1}(\omega)$  are always real, and these can be extended to the negative-frequency axis to be an even function of  $\omega$ . Therefore, these products can be formally treated as a differential operator similar to  $\varepsilon(i\partial_t)$  or  $\mu(i\partial_t)$ , provided that these are sufficiently regular in the frequency range under consideration.

We now introduce the following expression for the helicity density in the time domain:

$$\begin{aligned} \mathfrak{S}(\mathbf{r}, t) = \frac{1}{8\pi} \Big\{ & \mathcal{H}(\mathbf{r}, t) \cdot \mu(\mathbf{r}, i\partial_t) \mathcal{A}'(\mathbf{r}, t) - \mathcal{E}(\mathbf{r}, t) \cdot \varepsilon(\mathbf{r}, i\partial_t) \mathcal{C}'(\mathbf{r}, t) \\ & + \sum_n \sum_{m=1}^{2n} (-1)^{n+m} [\partial_t^{m-1} \mathcal{C}'(\mathbf{r}, t) \cdot \varepsilon_{2n}(\mathbf{r}) \partial_t^{2n-m+1} \mathcal{E}(\mathbf{r}, t) - \partial_t^{m-1} \mathcal{A}'(\mathbf{r}, t) \cdot \mu_{2n}(\mathbf{r}) \partial_t^{2n-m+1} \mathcal{H}(\mathbf{r}, t)] \Big\}. \end{aligned} \quad (14)$$

For monochromatic fields, when  $\mathcal{E}(\mathbf{r}, t) = \text{Re}[\mathbf{E}(\mathbf{r}, \omega)e^{-i\omega t}]$ , and similarly for  $\mathcal{H}$ ,  $\mathcal{A}'$ , and  $\mathcal{C}'$ , the time-averaged value of the helicity density (14) yields:

$$\mathfrak{S}(\mathbf{r}) = \frac{1}{16\pi} \text{Re} [\tilde{\mu}(\mathbf{r}, \omega) \mathbf{H}(\mathbf{r}, \omega)^* \cdot \mathbf{A}'(\mathbf{r}, \omega) - \tilde{\varepsilon}(\mathbf{r}, \omega) \mathbf{E}(\mathbf{r}, \omega)^* \cdot \mathbf{C}'(\mathbf{r}, \omega)]. \quad (15)$$

Furthermore, for monochromatic fields we have  $\mathbf{E} = i\omega \mathbf{A}$  and  $\mathbf{H} = i\omega \mathbf{C}$ , and the helicity density becomes:

$$\mathfrak{S} = g \text{Im} [-\tilde{\varepsilon} \nu Z \mathbf{E}^* \cdot \mathbf{H} + \tilde{\mu} \nu Z^{-1} \mathbf{H}^* \cdot \mathbf{E}], \quad (16)$$

which is exactly equivalent to Eq. (10) in the main text.

We now go back to the time-domain Eq. (14). We consider a medium with the following additional conditions:

$$\nabla(\nu Z) = \nabla(\nu Z^{-1}) = 0. \quad (17)$$

These correspond to a generalized homogeneity of the optical impedance (including the phase factor  $\nu$ ). Under conditions (17), it is possible to show that the time-domain helicity density (14) satisfies the following continuity equation (conservation law):

$$\partial_t \mathfrak{S}(\mathbf{r}, t) + \nabla \cdot \mathbf{\Sigma}(\mathbf{r}, t) = 0, \quad (18)$$

with the helicity flux

$$\mathbf{\Sigma}(\mathbf{r}, t) = \frac{1}{8\pi} [\mathcal{E}(\mathbf{r}, t) \times \mathcal{A}'(\mathbf{r}, t) + \mathcal{H}(\mathbf{r}, t) \times \mathcal{C}'(\mathbf{r}, t)]. \quad (19)$$

One can check the relation (18) using the identity

$$\partial_t \left[ \sum_n \sum_{m=1}^{2n} (-1)^{n+m} \partial_t^{m-1} \mathbf{F} \cdot \varepsilon_{2n} \partial_t^{2n-m} \mathbf{G} \right] = [\varepsilon(i\partial_t) \mathbf{F}] \cdot \mathbf{G} - \mathbf{F} \cdot [\varepsilon(i\partial_t) \mathbf{G}], \quad (20)$$

which can be verified by explicit (albeit lengthy) calculations.

For monochromatic fields, the helicity flux becomes:

$$\mathbf{\Sigma} = g \text{Im} (\nu Z^{-1} \mathbf{E}^* \times \mathbf{E} + \nu Z \mathbf{H}^* \times \mathbf{H}). \quad (21)$$

Notably, although in free space the helicity flux coincides with the spin angular momentum density  $\mathbf{S}$  [7–9], this is not the case in a medium,  $\mathbf{\Sigma} \neq \mathbf{S}$ , where the spin density is given in Eq. (5) of the main text [10, 11]. In the case of nondispersive materials (i.e.,  $\tilde{\mu} = \mu$  and  $\tilde{\varepsilon} = \varepsilon$ ), the helicity flux and the spin density are proportional to each other with a factor equal to the local refractive index:  $\mathbf{\Sigma} = \mathbf{S}/n$ . In the dispersive case, however, the helicity flux and the spin density are not directly related, since they depend on different medium parameters.

We also note that for nondispersive dielectric media, the helicity density (15), (16), and flux (21) coincide with the expression introduced by van Kruining and Götte [12]. Their treatment also allows extensions to some cases of bi-anisotropic media.

- 
- [1] S. Raghu and F. D. M. Haldane, Phys. Rev. A **78**, 033834 (2008).
  - [2] M. G. Silveirinha, Phys. Rev. B **92**, 125153 (2015).
  - [3] S. A. H. Gangaraj, M. G. Silveirinha, and G. W. Hanson, IEEE J. Multiscale and Multiphys. Comput. Techn. **2**, 3 (2017).
  - [4] G. D. Nittis and M. Lein, arXiv:1710.10148 (2017).
  - [5] D. C. Brody, J. Phys. A: Math. Theor. **47**, 035305 (2014).
  - [6] T. G. Philbin, Phys. Rev. A **87**, 043843 (2013).
  - [7] S. M. Barnett, R. P. Cameron, and A. M. Yao, Phys. Rev. A **86**, 013845 (2012).
  - [8] R. P. Cameron, S. M. Barnett, and A. M. Yao, New J. Phys. **14**, 053050 (2012).
  - [9] K. Y. Bliokh, A. Y. Bekshaev, and F. Nori, New J. Phys. **15**, 033026 (2013).
  - [10] K. Y. Bliokh, A. Y. Bekshaev, and F. Nori, Phys. Rev. Lett. **119**, 073901 (2017).
  - [11] K. Y. Bliokh, A. Y. Bekshaev, and F. Nori, New J. Phys. **19**, 123014 (2017).
  - [12] K. van Kruining and J. B. Götte, J. Opt. **18**, 085601 (2016).
